# Supplementary material for: Elite360D: Towards Efficient 360 Depth Estimation via Semantic- and Distance-Aware Bi-Projection Fusion
Source: arXiv:2403.16376 source file (2024-05-25)
Supplement: Supplementary file 1 [file X_suppl.tex]

\begin{abstract}
Due to the lack of space in the main paper, we provide more details of the proposed Elite360D and experimental results in the supplementary material. In Sec.~\ref{sec:supp_icosap}, we provide more prior knowledge of icosahedron projection (ICOSAP). In Sec.~\ref{sec:supp_network}, we provide a more detailed illustration of our network architecture. Sec.~\ref{sec:supp_loss} introduces our training loss functions and Sec.~\ref{sec:supp_dataset} introduces the used datasets and evaluation metrics in details. Moreover, we introduce the specific training details of prevalent methods and ERP-based depth baseline in Sec.~\ref{sec:supp_training_detail}, and we show additional quantitative and qualitative comparison results in Sec.~\ref{sec:supp_comparison_results}.
\end{abstract}
\section{Icosahedron Projection}
\label{sec:supp_icosap}
As shown in Fig.~\ref{fig:supp_ico}, with each increment in resolution on icosahedron projection (ICOSAP), each subdivision divides each equilateral triangle into 4 smaller equilateral triangles. We designate the initial icosahedron projection as $l=0$, where $l$ represents the level of subdivision. For different subdivision levels of the icosahedron projection, we can obtain corresponding faces ($f=20\times 4^{l}$) and vertices ($v=2+ 1\times 4^{l}$), as shown in Tab.~\ref{tab:sup_ico}. In the existing methods~\cite{Lee2018SpherePHDAC,Zhang2019OrientationAwareSS,Shakerinava2021EquivariantNF}, they focus on enable operations, \eg, convolution, pooling, and padding, on the ICOSAP. Specifically,~\cite{Zhang2019OrientationAwareSS} unfolds the ICOSAP onto the plane and aligns it to the standard image grid (See Fig.~\ref{fig:supp_ico_representation}(a)), while~\cite{Lee2018SpherePHDAC} represents 360$^\circ$ image as a SpherePHD version of geodesic icosahedron and directly presents the sphere convolution layers and pooling layers to process it (See Fig.~\ref{fig:supp_ico_representation}(b)). 
\begin{figure}[ht]
    \centering
    \resizebox{1\linewidth}{!}{ \includegraphics{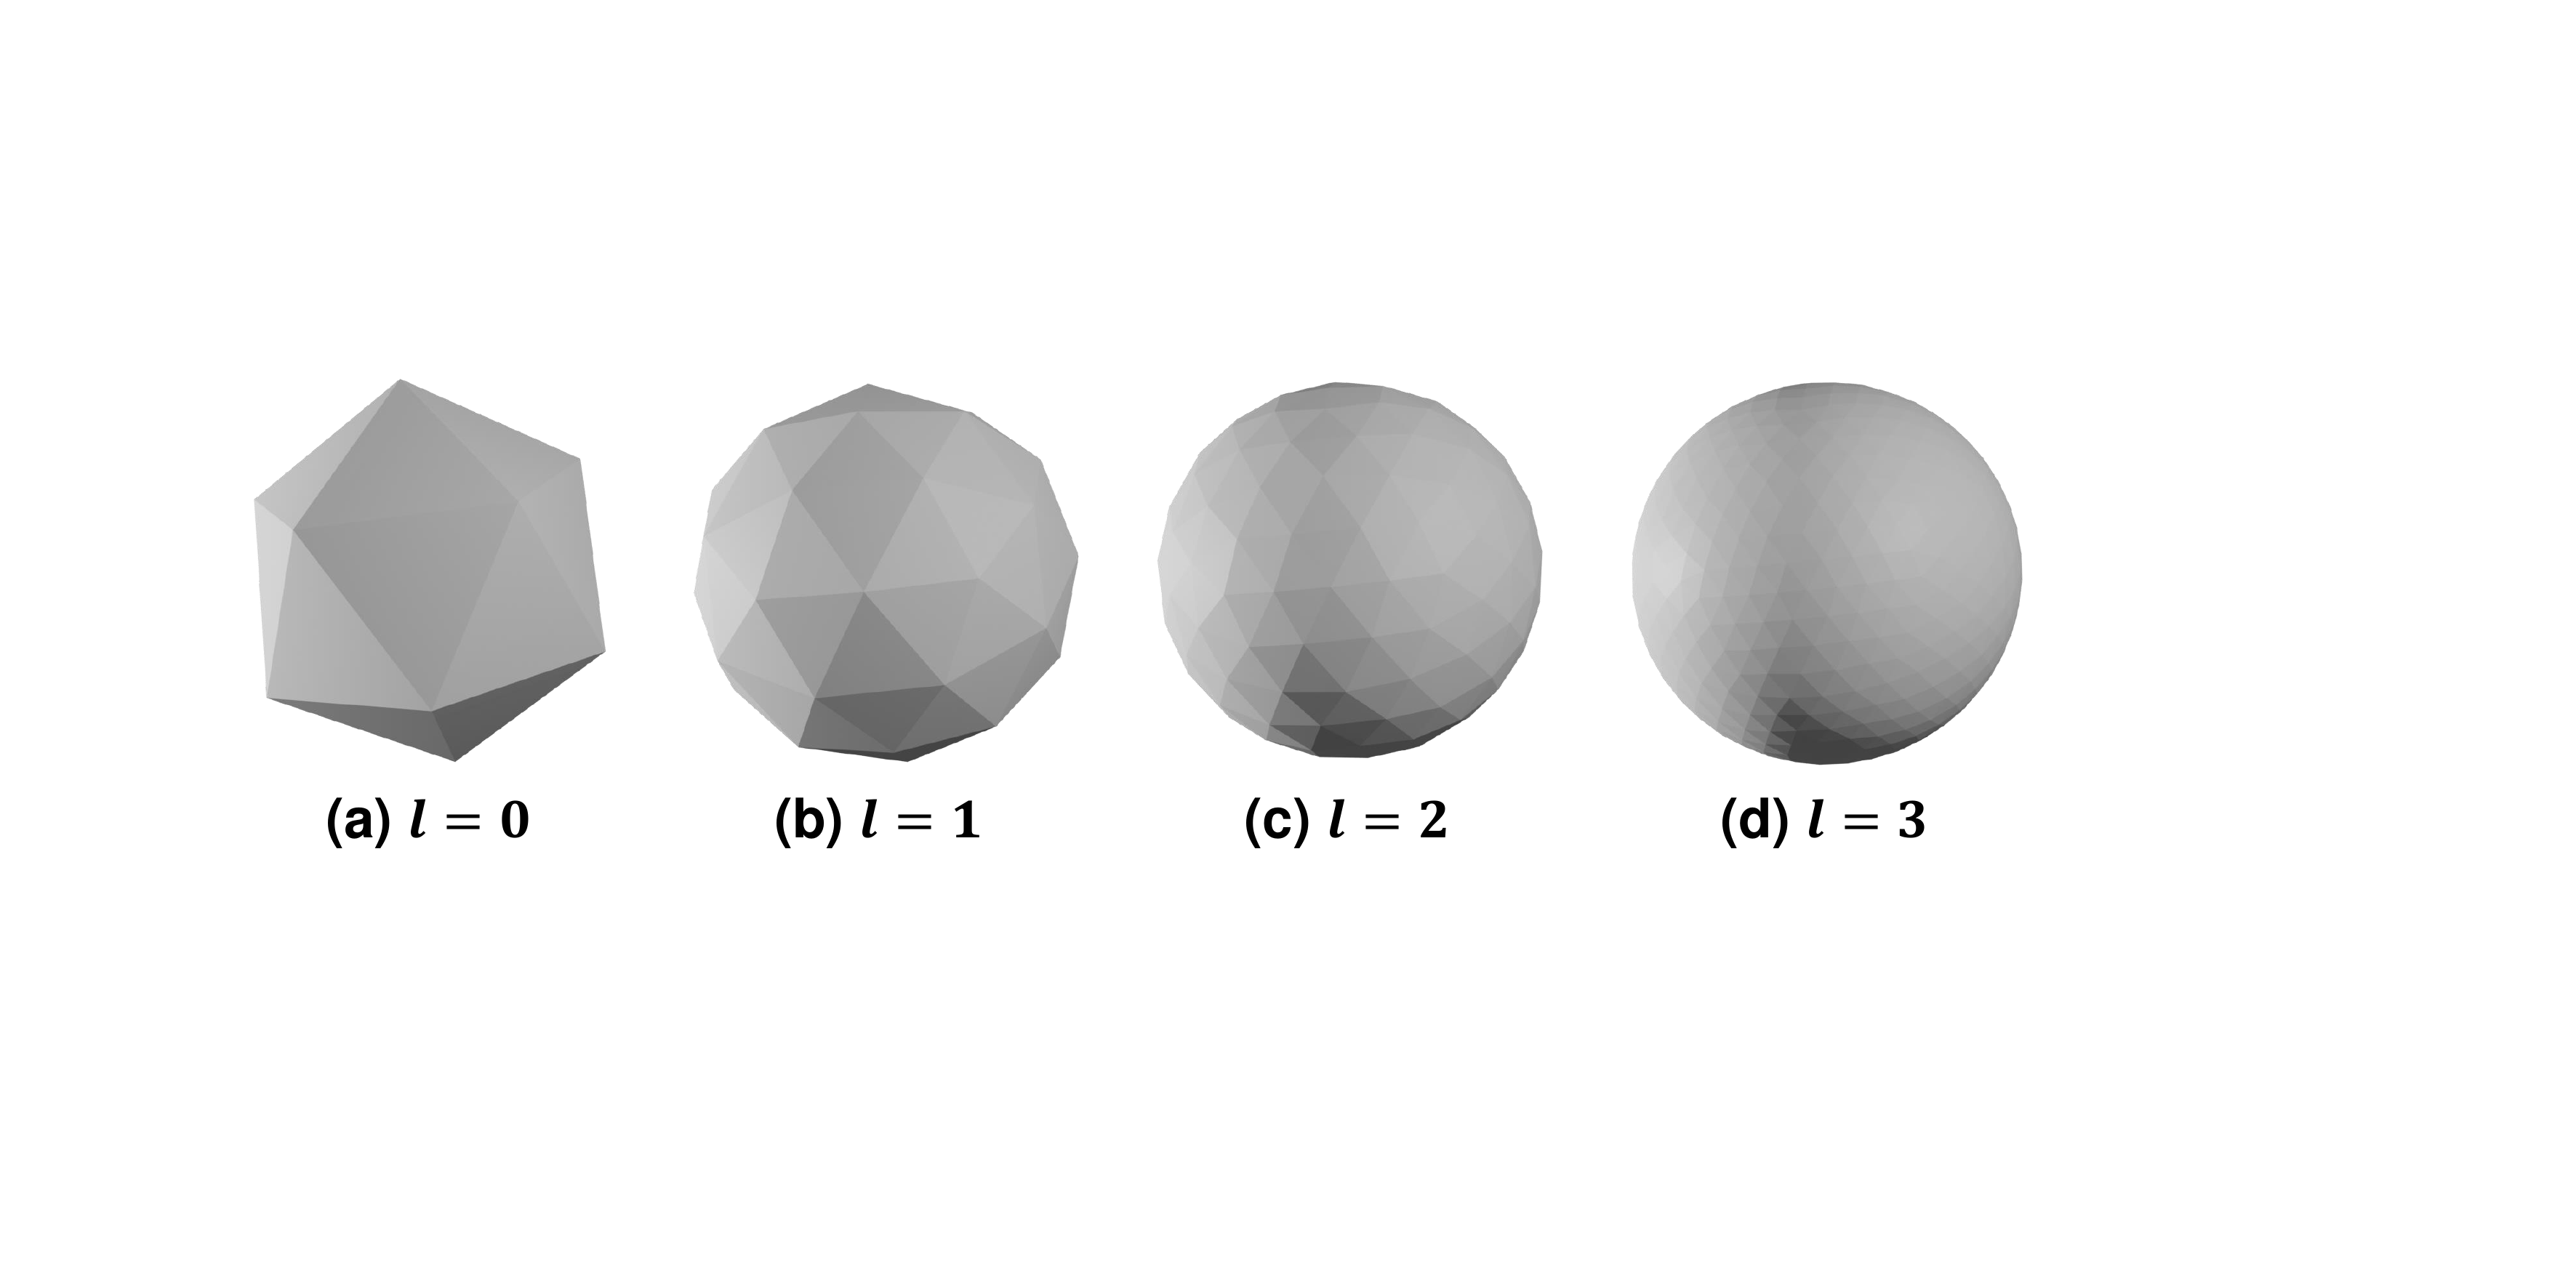}}
    \caption{The subdivision of icosahedron at different resolution $l$.}
    \label{fig:supp_ico}
\end{figure}
\begin{figure}[ht]
    \centering
    \resizebox{1\linewidth}{!}{ \includegraphics{sec/image/supp/sup_ico.pdf}}
    \caption{(a) Unfold representation (top) and image-grid-aligned representation (bottom) of ICOSAP. (b) icosahedral spherical polyhedron (SpherePHD) representation. (a), (b)are originally shown in~\cite{Zhang2019OrientationAwareSS} and~\cite{Lee2018SpherePHDAC}, respectively.}
    \label{fig:supp_ico_representation}
\end{figure}
\begin{table}[ht]
    \centering
    \resizebox{0.8\linewidth}{!}{ 
    \begin{tabular}{c|c|c|c}
    \toprule
     Resolution& $\#$Faces &$\#$Vertices&Each face\\
    \midrule
        $l=0$& 20 & 12 & \begin{minipage}[b]{0.3\columnwidth}
		\centering
		\raisebox{-.5\height}{\includegraphics[width=\linewidth]{sec/image/supp/ico_0.png}}
	\end{minipage}  \\
    \midrule
        $l=1$& 80 & 42 & \begin{minipage}[b]{0.3\columnwidth}
		\centering
		\raisebox{-.5\height}{\includegraphics[width=\linewidth]{sec/image/supp/ico_1.png}}
	\end{minipage}  \\
    \midrule
        $l=2$& 320 & 162 & \begin{minipage}[b]{0.3\columnwidth}
		\centering
		\raisebox{-.5\height}{\includegraphics[width=\linewidth]{sec/image/supp/ico_2.png}}
	\end{minipage}  \\
        \midrule
        $l=n$& $20\times 4^{n}$ & $2+10\times 4^{n}$ & $\cdots$ \\
    \bottomrule
    \end{tabular}}
    \caption{The subdivision of ICOSAP. The red points are the vertices and the original points are face centers.}
    \label{tab:sup_ico}
\end{table}
\begin{figure}[ht]
    \centering
    \resizebox{0.8\linewidth}{!}{ \includegraphics{sec/image/supp/sup_ico_center.pdf}}
    \caption{ICOSAP and corresponding face center point set.}
    \label{fig:supp_ico_center}
\end{figure}
\begin{figure*}[t]
    \centering
    \resizebox{1\textwidth}{!}{ \includegraphics{sec/image/supp/sup_network_architecture.pdf}}
    \caption{Overall Architecture of Elite360D.}
    \label{fig:supp_nework_achitecture}
\end{figure*}
\section{Details of Network Architecture}
\label{sec:supp_network}
In our Elite360D, for efficiency, we represent the ICOSAP data as the discrete point set. For better comprehension, we use a subdivision level $l=4$ as an example. Firstly, we create the subdivided icosahedron
with the $20 \times 4^{4} =5120 $ faces and $2+10 \times 4^4 = 2562$ vertices. Especially, as the vertices of the icosahedron lie on a spherical surface, we can calculate the RGB values of these vertices using the spherical spatial correspondence between the vertices and equirectangular projection (ERP) pixels. After obtaining the spatial coordinates $\left(x, y, z\right)$ of the vertices along with their RGB values, we can interpolate to obtain the coordinates and RGB values of the face centers. Since each face of the icosahedron is an equilateral triangle, we can directly calculate the averages of vertices for faces' coordinates and RGB values. Finally, we collect the $20 \times 4^{4} =5120$ face centers (See Fig.~\ref{fig:supp_ico_center}) and obtain the ICOSAP input tensors with the dimension of $\mathbb{R}^{5120 \times 6}$.

\begin{figure}[ht]
    \centering
    \resizebox{0.65\linewidth}{!}{ \includegraphics{sec/image/supp/sup_network_upsample.pdf}}
    \caption{Up-sample block in the decoder. $\bigoplus$ means the concatenation.}
    \label{fig:supp_nework_upsample}
\end{figure}

The overall network structure is described in Fig.~\ref{fig:supp_nework_achitecture}. The network comprises three main components: ERP feature extraction, ICOSAP feature extraction, and the B2F module. In most experimental setups, both ERP feature extraction and ICOSAP feature extraction have a channel number $C$ of 64. Similarly, the B2F module also operates with $d=64$ channels, except for the ResNet50 framework, which employs 256 channels, and the Swin-B framework, which uses 128 channels. Especially, for ERP feature extraction, we directly employ the 2D models, which are designed for perspective images and pre-trained on large-scale ImageNet~\cite{JiaDeng2009ImageNetAL} dataset. For ICOSAP feature extraction, we directly employ the encoder in Point Transformer~\cite{Zhao2020PointT} with three transition down blocks as the point feature extractor. Especially, for the decoding stage, we employ common skip-connections and utilize the fused feature $F^{GL}$ along with multi-scale ERP-based encoded features to jointly predict the final depth. In Fig.~\ref{fig:supp_nework_upsample}, we illustrate the details of the up-sampling block.

\section{Training Loss}
\label{sec:supp_loss}
For the depth supervision, we follow existing works~\cite{Shen2022PanoFormerPT, Pintore2021SliceNetDD} and employ the combination of Berhu loss~\cite{Laina2016DeeperDP} and gradient loss~\cite{Pintore2021SliceNetDD}.
\begin{equation}
\small
\begin{gathered}
\mathcal{L}_{total}=\mathcal{L}_{depth}+\mathcal{L}_{grad},\\ 
\mathcal{L}_{depth} = \sum_{i\in P}\mathcal{B}(D^i- D^i_{GT}),\\
\mathcal{L}_{grad} =\mathcal{B}(\nabla_x D- \nabla_x D_{GT})+\mathcal{B}(\nabla_y D- \nabla_y D_{GT}),
\end{gathered}
\label{eq:gate_fusion}
\end{equation}
where $\mathcal{B}$ is the Berhu loss~\cite{Laina2016DeeperDP}, which is formulated as:
\begin{align}
    \mathcal{B}(x)=\left\{\begin{aligned}	
		&\left | x\right |, \left | x\right |\leq c\\
		&\frac{x^2+c^2}{2c}, \left | x\right | > c\\
	\end{aligned}\right.
\end{align}
$D$ is the depth prediction, $D_{GT}$ is the ground truth, $P$ indicates pixels which are valid in the ground truth, $\nabla_x$ denotes the horizontal derivatives and $\nabla_y$ denotes the vertical ones. $c$ is a threshold hyper-parameter and set to 0.2 empirically~\cite{Li2022OmniFusion3M,Jiang2021UniFuseUF}. To obtain the gradients $\nabla_x$ and $\nabla_y$, we follow PanoFormer~\cite{Shen2022PanoFormerPT} to use two convolution kernels. 
\begin{table}[t]
    \centering
    \resizebox{1\linewidth}{!}{ 
    \begin{tabular}{c|c|c|c}
    \toprule
    Datasets&Matterport3D& Stanford2D3D&Structure3D\\
    \midrule
    $\#$train& 7829& 1040 & 18343\\
    $\#$val& 957& - & 1776\\
    $\#$test&  2014&373 & 1697\\
    \bottomrule
    \end{tabular}}
    \caption{The statistics of the datasets.}
    \label{tab:sup_dataset}
\end{table}

\begin{figure}[t]
    \centering
    \resizebox{1\linewidth}{!}{ \includegraphics{sec/image/supp/sup_dataset.pdf}}
    \caption{Examples of three datasets: (a) Matterport3D, (b) Stanford2D3D, and (c) Structure3D.}
    \label{fig:supp_dataset}
\end{figure}

\section{Datasets and Evaluation Metrics}
\label{sec:supp_dataset}
\noindent \textbf{Datasets.} We evaluate our methods on three popular datasets: Matterport3D~\cite{Chang2017Matterport3DLF}, Stanford2D3D~\cite{Armeni2017Joint2D} and Structure3D~\cite{Zheng2019Structured3DAL}. Matterport3D and Stanford2D3D are real-world datasets, while Structure3D is a synthetic dataset. The statics of three datasets are listed in Tab.~\ref{tab:sup_dataset}. Matterport3D totally contains 10,800 ERP images, including 7,829 samples for training, 957 samples for validation, and 2014 samples for testing. Stanford2D3D is a small-scale indoor dataset, which only contains 1413 samples (1040 training samples and 373 testing samples). For Structure3D, a recently proposed large-scale synthetic dataset, it includes 18343 training samples, 1776 validation samplings, and 1697 testing samples. During training and testing, we set the resolutions of all samples as $512 \times 1024$. The examples of three datasets are illustrated in Fig.~\ref{fig:supp_dataset}.

\noindent \textbf{Evaluation metrics.} For the evaluation metrics, we adopted widely used metrics from 360 depth estimation methods, such as BiFuse~\cite{Wang2020BiFuseM3}, UniFuse~\cite{Jiang2021UniFuseUF}, and HRDFuse~\cite{Ai2023HRDFuseM3}. These metrics include three error metrics: absolute relative error (Abs Rel), squared relative error (Sq Rel), root mean squared error (RMSE), and three threshold percentage $\delta<\alpha^{t}$ $(\alpha=1.25, t=1,2,3)$, denoted as $\delta_{t}$. Particularly noteworthy is that, for all metric computations, we employed the common practice of considering only valid pixels~\cite{Jiang2021UniFuseUF,Ai2023HRDFuseM3}\footnote{\url{https://github.com/alibaba/UniFuse-Unidirectional-Fusion/}}. However, this differs from the approach taken in original PanoFormer~\footnote{\url{https://github.com/zhijieshen-bjtu/PanoFormer}}.

\section{Training Details}
\label{sec:supp_training_detail}
Considering that existing methods have varied training settings, \eg, optimizer, learning rate scheduler, final depth prediction, loss function and number of training epochs. Therefore, in this study, for a fair comparison and to better assess the effectiveness of different methods, we re-trained all methods using their official codes and standardized training settings. Specifically, for the optimizer, we followed UniFuse~\cite{Jiang2021UniFuseUF} and used the Adam optimizer~\cite{Kingma2014AdamAM} with default settings. Meanwhile, we also followed UniFuse to avoid any learning rate scheduler. For the final depth prediction, We first utilized the sigmoid function to output depth probabilities, which are then multiplied by the maximum depth value to obtain the final depth values.
Regarding the loss function, we followed PanoFormer~\cite{Shen2022PanoFormerPT}, utilizing the combination of Berhu loss along with gradient loss. To ensure convergence for each method, we trained all methods for 200 epochs on Matterport3D and Stanford2D3D datasets and 60 epochs on Structure3D dataset, following the setting in PanoFormer. For the ERP-based depth baseline, we directly removed the ICOSAP feature extraction and B2F module in Fig.~\ref{fig:supp_nework_achitecture}. We employed the encoder-decoder based network to directly predict the depth values form the ERP input.

\section{Additional Quantitative and Qualitative Results}
\label{sec:supp_comparison_results}
\noindent \textbf{More quantitative results.} In Table.~\ref{tab:supp_comparison}, we present more comparison results with the ERP baseline, while employing the various encoder backbones. We can observe that our Elite3D outperforms the ERP baseline significantly on the Stanford2D3D and Structure3D datasets, while incurring only minimal computational cost. 
\begin{table*}[ht]
    \centering
    \resizebox{0.95\textwidth}{!}{ 
    \begin{tabular}{c|c|c|c|c|c|c|c|c|c|c}
    \toprule[1pt]
    Datasets&Backbone& Method&$\#$Params (M)&$\#$FLOPs (G)& Abs Rel $\downarrow$& Sq Rel $\downarrow$&RMSE $\downarrow$ &$\delta_1 (\%)$ $\uparrow$ & $\delta_2 (\%)$ $\uparrow$ & $\delta_3 (\%)$ $\uparrow$\\
    \midrule[1pt]
    \multirow{12}*{S2D3D~\cite{Armeni2017Joint2D}}& \multirow{3}*{ResNet-18~\cite{He2015DeepRL}}&Equi-Baseline& 14.39 &39.84 & 0.1357 & 0.0855 &0.4066 & 84.46 &95.54 & 98.40 \\
      & &Ours& 15.43 & 45.91 & 0.1321 &  0.0838 & 0.3958 & 86.01 & 95.69 & 98.52 \\
      & &\cellcolor{gray!40}$\varDelta$&\cellcolor{gray!40}+1.04& \cellcolor{gray!40}+6.07& \cellcolor{gray!40}\textbf{-2.65$\%$}&\cellcolor{gray!40}\textbf{-1.99$\%$} &\cellcolor{gray!40}\textbf{-2.66$\%$} & \cellcolor{gray!40}\textbf{+1.55}& \cellcolor{gray!40}\textbf{+0.15}& \cellcolor{gray!40}\textbf{+0.12} \\
      \cmidrule{2-11}
      & \multirow{3}*{ResNet-34~\cite{He2015DeepRL}}&Equi-Baseline&24.50 & 59.22 & 0.1203& 0.0754 & 0.3724& 87.41 & 96.51& 98.77\\
      & &Ours&25.51 & 65.28 & 0.1182& 0.0728&0.3756 &88.72 &96.84 & 98.92\\
      & &\cellcolor{gray!40}$\varDelta$&\cellcolor{gray!40}+1.01& \cellcolor{gray!40}+6.06& \cellcolor{gray!40}\textbf{-9.21$\%$}&\cellcolor{gray!40}\textbf{-3.45$\%$} &\cellcolor{red!10}{\textbf{\textcolor{red}{+0.86$\%$}}} & \cellcolor{gray!40}\textbf{+1.31}& \cellcolor{gray!40}\textbf{+0.33}& \cellcolor{gray!40}\textbf{+0.15} \\
      \cmidrule{2-11}
      & \multirow{3}*{ResNet-50$^*$~\cite{He2015DeepRL}}&Equi-Baseline&29.63 &75.13 & 0.1319 & 0.0894 & 0.4020 & 83.80 & 95.39 & 98.38\\
      & &Ours&42.99 & 170.11 &0.1121 & 0.0769 & 0.3693& 88.11& 96.29& 98.85\\
      & &\cellcolor{gray!40}$\varDelta$&\cellcolor{gray!40}+13.36& \cellcolor{gray!40} +94.98& \cellcolor{gray!40}\textbf{-15.01$\%$}&\cellcolor{gray!40}\textbf{-13.98$\%$} &\cellcolor{gray!40}\textbf{-8.13$\%$} & \cellcolor{gray!40}\textbf{+4.38}& \cellcolor{gray!40}\textbf{+0.90}& \cellcolor{gray!40}\textbf{+0.47} \\
      \cmidrule{2-11}
      & \multirow{3}*{EfficientNet-B5~\cite{Tan2019EfficientNetRM}}&Equi-Baseline & 3.10& 18.81 & 0.1026&0.0638 &0.3580 & 89.43 & 97.06& 99.16\\
      & &Ours&4.11 & 24.88& 0.1018 &0.0603 & 0.3575& 89.47&97.23 &99.22 \\
      & &\cellcolor{gray!40}$\varDelta$& \cellcolor{gray!40}+1.01& \cellcolor{gray!40}+6.07& \cellcolor{gray!40}\textbf{-0.78$\%$}&\cellcolor{gray!40}\textbf{-5.49$\%$} &\cellcolor{gray!40}\textbf{-0.14$\%$} & \cellcolor{gray!40}\textbf{+0.03}& \cellcolor{gray!40}\textbf{+0.17}& \cellcolor{gray!40}\textbf{+0.06} \\
      \midrule[1pt]
      \multirow{12}*{Struct3D~\cite{Zheng2019Structured3DAL}}&\multirow{3}*{ResNet-18~\cite{He2015DeepRL}}&Equi-Baseline&14.39 &39.84& 0.3005&0.5730 &0.9792&67.85 &85.20&91.94 \\
      & &Ours& 15.43 & 45.91&0.1775&0.2571&0.5989&82.73&93.41&96.70 \\
      & &\cellcolor{gray!40}$\varDelta$&\cellcolor{gray!40}+1.04& \cellcolor{gray!40}+6.07& \cellcolor{gray!40}\textbf{-40.93$\%$}&\cellcolor{gray!40}\textbf{-55.13$\%$} &\cellcolor{gray!40}\textbf{-38.84$\%$} & \cellcolor{gray!40}\textbf{+14.88}& \cellcolor{gray!40}\textbf{+8.21}& \cellcolor{gray!40}\textbf{+4.76} \\
      \cmidrule{2-11}
      &\multirow{3}*{ResNet-34~\cite{He2015DeepRL}}&Equi-Baseline&24.50 &59.22& 0.2256&0.3910 &0.7641&76.90 &89.96 &94.49 \\
      & &Ours& 25.51&65.28&0.1480&0.2215&0.4961&87.41&94.34&96.66 \\
      & &\cellcolor{gray!40}$\varDelta$& \cellcolor{gray!40}+1.01& \cellcolor{gray!40}+6.06& \cellcolor{gray!40}\textbf{-34.40$\%$}&\cellcolor{gray!40}\textbf{-43.35$\%$} &\cellcolor{gray!40}\textbf{-35.07$\%$} & \cellcolor{gray!40}\textbf{+10.51}& \cellcolor{gray!40}\textbf{+4.38}& \cellcolor{gray!40}\textbf{+2.17} \\
      \cmidrule{2-11}
      &\multirow{3}*{ResNet-50~\cite{He2015DeepRL}}&Equi-Baseline&29.63 &75.13&0.2814& 0.5125&0.9449& 68.94&86.41& 92.77\\
      & &Ours& 42.99 & 170.11& 0.1485&0.2270& 0.4858&87.54&94.75&96.86 \\
      & &\cellcolor{gray!40}$\varDelta$&\cellcolor{gray!40}+13.36& \cellcolor{gray!40} +94.98& \cellcolor{gray!40}\textbf{-47.23$\%$}&\cellcolor{gray!40}\textbf{-55.70$\%$} &\cellcolor{gray!40}\textbf{-48.59$\%$} & \cellcolor{gray!40}\textbf{+18.60}& \cellcolor{gray!40}\textbf{+8.34}& \cellcolor{gray!40}\textbf{+4.09} \\
      \cmidrule{2-11}
      & \multirow{3}*{EfficientNet-B5~\cite{Tan2019EfficientNetRM}}&Equi-Baseline&3.10&18.81 &0.1312 & 0.1938& 0.4312&88.53 &95.21 &97.40 \\
      & &Ours&4.11& 24.88 &0.1277 &0.1930 &0.4151 & 89.16&95.33 &97.43 \\
      &&\cellcolor{gray!40}$\varDelta$&\cellcolor{gray!40}+1.01& \cellcolor{gray!40}+6.07& \cellcolor{gray!40}\textbf{-2.67$\%$}&\cellcolor{gray!40}\textbf{-0.41$\%$} &\cellcolor{gray!40}\textbf{-3.73$\%$} & \cellcolor{gray!40}\textbf{+0.63}& \cellcolor{gray!40}\textbf{+0.12}& \cellcolor{gray!40}\textbf{+0.03} \\
      \bottomrule[1pt]
    \end{tabular}}
    \caption{\textbf{Quantitative comparison with ERP-based depth baseline}. For most conditions, we set the channel number $C$ to 64. Especially, we set $C$ to 256 for ResNet-50$^*$ and to 128 for Swin-B$^*$. \textbf{Bold} indicates performance improvement. \colorbox{red!10}{\textcolor{red}{\textbf{Red}}} indicates performance decline.}
    \label{tab:supp_comparison}
\end{table*}

We examine the generalization capability of different models via training on Matterport3D training dataset and testing on Stanford2D3D test dataset. As the sensing depth of Matterport3D does not cover the top and bottom of the panorama, to make a fair comparison, we do not count the topmost and lowest 68 pixels following UniFuse~\cite{Jiang2021UniFuseUF} when evaluating on Stanford2D3D. The results are shown in~Table.~\ref{tab:supp_generalization}. Under the condition of using ResNet34 as the ERP encoder backbone, we can see that OmniFusion achieves the best results on all evaluation metrics. Simultaneously, our Elite360 model, with just an about additional 1M parameters, secures the second-best performance across most metrics. Especially, with the EfficientNet-B5 as the encoder backbone, our Elite360D significantly outperforms existing methods on all evaluation metrics.
\noindent \textbf{About the inference time.} We count the inference time in Table.~\ref{tab:supp_inference_time} for Elite360D, ERP depth baseline, and prevalent methods. Especially, we show the results of frames per second (FPS) with ResNet-34 as the backbone. The inference time includes the projection processing time. Besides, we calculated the average preparation time for each ICOSAP point set to be 0.25s.

\begin{table*}[ht]
    \centering
    \resizebox{0.95\textwidth}{!}{ 
    \begin{tabular}{c|c|c|c|c|c|c|c|c|c|c}
    \toprule[1pt]
    Datasets&Backbone& Method&$\#$Params (M)&$\#$FLOPs (G)& Abs Rel $\downarrow$& Sq Rel $\downarrow$&RMSE $\downarrow$ &$\delta_1 (\%)$ $\uparrow$ & $\delta_2 (\%)$ $\uparrow$ & $\delta_3 (\%)$ $\uparrow$\\
    \midrule[1pt]
    \multirow{8}*{ \makecell[c]{Train on M3D~\cite{Chang2017Matterport3DLF}\\ test on S2D3D~\cite{Armeni2017Joint2D}}}& \multirow{5}*{ResNet-34~\cite{He2015DeepRL}}&Equi-Baseline& 24.50 & 59.22 & 0.1525& 0.1203 &0.4640 & 81.61 &95.08 & 98.36 \\
    & &BiFuse& 56.01 &199.58 & 0.1349&	0.1052	& 0.4317 &86.06	&	95.90&	98.39 \\
    & &UniFuse& 50.48& 96.52 & 0.1382 &  0.1030 & 0.4383 & 81.64 & 95.56 & \cellcolor{yellow!40}{98.64} \\
    & &OmniFusion& 42.46& 142.29& \cellcolor{gray!40}{0.1208}&\cellcolor{gray!40}{0.0894}&\cellcolor{gray!40}{0.4117}&\cellcolor{gray!40}{86.90}& \cellcolor{gray!40}{96.41}& \cellcolor{gray!40}{98.69}\\
      & &Ours& 25.51 & 65.28 &\cellcolor{yellow!40}{0.1305}&	\cellcolor{yellow!40}{0.0985}&	\cellcolor{yellow!40}{0.4247}&	\cellcolor{yellow!40}{86.15}&\cellcolor{yellow!40}{96.16}&{98.52}\\
      \cmidrule{2-11}
    & Transformer&PanoFormer~\cite{Shen2022PanoFormerPT}& 20.38& 81.09  &0.1261	&0.0960&0.4137&86.63&96.48&98.54\\
      & Transformer&EGFormer~\cite{Yun2023EGformerEG}& 15.39&66.21&0.1902&0.1887&0.5813&75.89&91.95&97.59\\
    \cmidrule{2-11}
      & \multirow{2}*{EfficientNet-B5~\cite{Tan2019EfficientNetRM}}& Equi-Baseline & 4.11 &24.88& 0.1161& 0.0785 &0.3790 & 88.82 &96.90 & 98.76\\
      
      & &Ours & 4.11 &24.88& \textcolor{green}{0.1022}& \textcolor{green}{0.0674} &\textcolor{green}{0.3715} & \textcolor{green}{89.44} &\textcolor{green}{97.40} & \textcolor{green}{99.16}\\
      
      \bottomrule[1pt]
    \end{tabular}}
    \caption{\textbf{Generalization comparison with SOTA methods}. We train all the models on Matterport3D training dataset and test the models on Stanford2D3D test dataset. \textcolor{green}{Green} means the best performance among all methods. \colorbox{gray!40}{{Gray box}} indicates the best performance with ResNet-34 as the ERP encoder and \colorbox{yellow!40}{{yellow box}} indicates the second best performance with ResNet-34 as the ERP encoder.}
    \label{tab:supp_generalization}
\end{table*}
\begin{table*}[h]

\scriptsize
    \centering
    \vspace{-10pt}
    \resizebox{0.9\columnwidth}{!}{
    \begin{tabular}{cccccc}
    \toprule
    & ERP& BiFuse& UniFuse &OmniFusion& Elite360D \\
    \cmidrule{1-6}
    FPS& 9.15 &1.27 &2.06& 1.55 &3.81\\
    \bottomrule
    \end{tabular}}
    \vspace{-9pt}
    \caption{Inference time comparison results.}
    \label{tab:supp_inference_time}
    \vspace{-12pt}
\end{table*}

\begin{figure*}[ht]
    \centering
    \resizebox{0.95\linewidth}{!}{ \includegraphics{sec/image/supp/supp_matterport.pdf}}
    \caption{Visual comparisons on Matterport3D dataset.}
    \label{fig:supp_matterport}
\end{figure*}

\begin{figure*}[ht]
    \centering
    \resizebox{0.95\linewidth}{!}{ \includegraphics{sec/image/supp/supp_stanford.pdf}}
    \caption{Visual comparisons on Stanford2D3D dataset.}
    \label{fig:supp_stanford}
\end{figure*}

\begin{figure*}[ht]
    \centering
    \resizebox{0.95\linewidth}{!}{ \includegraphics{sec/image/supp/supp_structure.pdf}}
    \caption{Visual comparisons on Structure3D dataset.}
    \label{fig:supp_structure}
\end{figure*}
\noindent \textbf{More qualitative results.}
In Fig.~\ref{fig:supp_matterport},~\ref{fig:supp_stanford} and~\ref{fig:supp_structure}, we showcase visual comparisons on the Matterport3D, Stanford2D3D, and Structure3D datasets, respectively. It's evident that our Elite360D predicts depth values more accurately, particularly on wall surfaces and certain architectural details.
\clearpage
